# Supplementary material for: An Adaptive Gas Cost Mechanism for Ethereum to Defend Against Under-Priced DoS Attacks
Source: arXiv:1712.06438 source file (2020-11-04)
Supplement: Supplementary file 1 [file appendix.tex]

\appendix
\section{An expensive path and a cheap path of \emph{opSuicide}}
\label{appendix-path}

\section{Execution time of representative EVM operations}
\label{appendix-time}

\section{Handlers for \texttt{DIV} and \texttt{SDIV}}
\label{appendix-source}

\section{Curves of Eqn. (\ref{eq_gas})}
\label{appendix-curve}

\section{Average number of executions of EVM operations}
\label{appendix-ave}
